# Supplementary material for: Sine-skewed toroidal distributions and their application in protein bioinformatics
Source: arXiv:1910.13293 source file (2019-10-29)
Supplement: Supplementary file 1 [file SM_sine_skewed_v3.pdf]

# Sine-skewed toroidal distributions and their application in protein bioinformatics: Supplementary Material

Jose Ameijeiras-Alonso<sup>1,\*</sup> and Christophe Ley<sup>2,†</sup>

\*KU Leuven and <sup>†</sup>Ghent University

## Abstract

Section S1 includes the needed proofs for deriving some of the properties shown in the main paper. Extra results regarding the protein data are provided in Section S2. In particular, for the amino acid types that are not analyzed in the main paper, this section contains extra tables and figures showing the achieved fitting when using different toroidal distributions and their sine-skewed versions.

*Keywords:* Directional Statistics; Flexible Modeling; Skewness; Structural Bioinformatics; Toroidal Data.

## S1 Proofs of Section 2

### S1.1 Marginals

Assume, without loss of generality, that  $\mu = \mathbf{0}$ . Given the subset  $\mathbf{m} \subset \{1, \dots, d\}$  and denoting by  $g_{\mathbf{m}}$  the marginal density of  $\mathbf{X}_{\mathbf{m}}$ , we have, both if  $f$  is pointwise symmetric in  $\mathbf{x}_{\mathbf{m}^c} = \{x_s : s \in \mathbf{m}^c\}$  alone (while fixing the other components) or if  $\lambda_s = 0$  for all  $s \in \mathbf{m}^c$ , that

---

<sup>1</sup>Supported by the FWO research project G.0826.15N (Flemish Science Foundation), GOA/12/014 project (Research Fund KU Leuven), Project MTM2016-76969-P from the Spanish State Research Agency (AEI) co-funded by the European Regional Development Fund (ERDF) and the Competitive Reference Groups 2017-2020 (ED431C 2017/38) from the Xunta de Galicia through the ERDF.

<sup>2</sup>Supported by the FWO Krediet aan Navorsers grant with reference number 1510391N.

$$\begin{aligned}
g_{\mathbf{m}}(x_{\mathbf{m}}; \boldsymbol{\vartheta}, \boldsymbol{\lambda}_{\mathbf{m}}) &= \int_{-\pi}^{\pi} \cdots \int_{-\pi}^{\pi} f(\mathbf{x}; \boldsymbol{\vartheta}) \left( 1 + \sum_{s=1}^d \lambda_s \sin(x_s) \right) dx_{\mathbf{m}^c} \\
&= f_{\mathbf{m}}(\mathbf{x}_{\mathbf{m}}; \boldsymbol{\vartheta}) \left( 1 + \sum_{s \in \mathbf{m}} \lambda_s \sin(x_s) \right) + \sum_{s \in \mathbf{m}^c} \lambda_s \left( \int_0^{\pi} \cdots \int_0^{\pi} \sin(x_s) f(\mathbf{x}; \boldsymbol{\vartheta}) dx_{\mathbf{m}^c} \right. \\
&\quad \left. + \int_0^{\pi} \cdots \int_0^{\pi} \sin(-x_s) f(-\mathbf{x}; \boldsymbol{\vartheta}) dx_{\mathbf{m}^c} \right) \\
&= f_{\mathbf{m}}(\mathbf{x}_{\mathbf{m}}; \boldsymbol{\vartheta}) \left( 1 + \sum_{s \in \mathbf{m}} \lambda_s \sin(x_s) \right),
\end{aligned}$$

where  $f_{\mathbf{m}}$  stands for the marginal density of  $f$  with respect to the components in  $\mathbf{m}$ .

## S1.2 Trigonometric moments and shape parameters

In the following, given the trigonometric moments of any base density, we derive the trigonometric moments for its sine-skewed version:

$$\begin{aligned}
\alpha_{\mathbf{p}} &= \int_{-\pi}^{\pi} \cdots \int_{-\pi}^{\pi} \cos(p_1 x_1 + \dots + p_d x_d) f(\mathbf{x}; \boldsymbol{\vartheta}) \left( 1 + \sum_{s=1}^d \lambda_s \sin(x_s) \right) d\mathbf{x} \\
&= \int_{-\pi}^{\pi} \cdots \int_{-\pi}^{\pi} \cos(p_1 x_1 + \dots + p_d x_d) f(\mathbf{x}; \boldsymbol{\vartheta}) d\mathbf{x} = \alpha_{\mathbf{p}}^0; \\
\beta_{\mathbf{p}} &= \int_{-\pi}^{\pi} \cdots \int_{-\pi}^{\pi} \sin(p_1 x_1 + \dots + p_d x_d) f(\mathbf{x}; \boldsymbol{\vartheta}) \left( 1 + \sum_{s=1}^d \lambda_s \sin(x_s) \right) d\mathbf{x} \\
&= \sum_{s=1}^d \frac{\lambda_s}{2} \int_{-\pi}^{\pi} \cdots \int_{-\pi}^{\pi} [\cos(p_1 x_1 + \dots + p_{s-1} x_{s-1} + (p_s - 1)x_s + p_{s-1} x_{s-1} + \dots + p_d x_d) \\
&\quad - \cos(p_1 x_1 + \dots + p_{s-1} x_{s-1} + (p_s + 1)x_s + p_{s-1} x_{s-1} + \dots + p_d x_d)] f(\mathbf{x}; \boldsymbol{\vartheta}) d\mathbf{x} \\
&= \frac{1}{2} \sum_{s=1}^d \lambda_s \left( \alpha_{[p_1, \dots, p_{s-1}, (p_s-1), p_{s+1}, \dots, p_d]}^0 - \alpha_{[p_1, \dots, p_{s-1}, (p_s+1), p_{s+1}, \dots, p_d]}^0 \right).
\end{aligned}$$

Here we made use of symmetry arguments as well as trigonometric identities. The values of the second cosine and sine moments about the mean direction, needed for computing the skewness and kurtosis parameters, can be obtained from the previous values using the following identities:

$$\begin{aligned}
\bar{\beta}_{2\mathbf{e}_s} &= \mathbb{E}[\sin 2(X_s - \mu_{1;s})] \\
&= (\cos^2(\mu_{1;s}) - \sin^2(\mu_{1;s})) \mathbb{E}[\sin(2X_s)] - 2 \sin(\mu_{1;s}) \cos(\mu_{1;s}) \mathbb{E}[\cos(2X_s)], \\
\rho_{1;s}^2 \bar{\beta}_{2\mathbf{e}_s} &= \beta_{2\mathbf{e}_s} (\alpha_{\mathbf{e}_s}^2 - \beta_{\mathbf{e}_s}^2) - 2 \alpha_{2\mathbf{e}_s} \beta_{\mathbf{e}_s} \alpha_{\mathbf{e}_s}, \\
\rho_{1;s}^2 \bar{\alpha}_{2\mathbf{e}_s} &= \alpha_{2\mathbf{e}_s} (\alpha_{\mathbf{e}_s}^2 - \beta_{\mathbf{e}_s}^2) + 2 \beta_{2\mathbf{e}_s} \beta_{\mathbf{e}_s} \alpha_{\mathbf{e}_s}.
\end{aligned}$$

### S1.3 Random number generation

Consider the random variable  $Y$  with associated density function  $f(\cdot - \mu; \vartheta)$  symmetric around  $\mu$ , and  $U$  following a uniform distribution on  $[0, 1]$ . Consider the random variable

$$X = \begin{cases} Y & \text{if } U \leq \left(1 + \sum_{s=1}^d \lambda_s \sin(Y_s - \mu_s)\right) / 2 \\ -Y + 2\mu & \text{if } U > \left(1 + \sum_{s=1}^d \lambda_s \sin(Y_s - \mu_s)\right) / 2. \end{cases}$$

The associated density of  $X$  at a point  $x$  is given by

$$\frac{1}{2}f(x - \mu; \vartheta) \left(1 + \sum_{s=1}^d \lambda_s \sin(x_s - \mu_s)\right) + \frac{1}{2}f(-x + \mu; \vartheta) \left(1 - \sum_{s=1}^d \lambda_s \sin(-x_s + \mu_s)\right).$$

Since  $\sin(x_s - \mu_s) = -\sin(-x_s + \mu_s)$  and  $f(x - \mu; \vartheta) = f(-x + \mu; \vartheta)$ , the latter expression yields the desired density function (2.1).

## S2 Further details on the analysis of the protein data

In this section, we include the extra results related to the 17 different amino acid types that are not included in the main paper. This section contains six tables, Tables S1-S6, providing, for every amino acid type, the MLEs of the mixtures of different base densities (the bivariate Sine, Cosine and wrapped Cauchy distributions) and the mixtures of their sine-skewed versions. Tables S1-S6 thus contain the estimated parameters, log-likelihood, AIC, BIC values and indicate when the null hypothesis of symmetry was rejected at significance level  $\alpha = 0.01$  for each model. Finally, the Ramachandran plots of the different amino acid type data and maximum likelihood fits of the different models are provided in Figures S1-S6.

|                 | Model | Comp | $\hat{\mu}_1$ | $\hat{\mu}_2$ | $\hat{\kappa}_1$ | $\hat{\kappa}_2$ | $\hat{r}$ | $\hat{\lambda}_1$ | $\hat{\lambda}_2$ | $\hat{p}$ | LL      | AIC    | BIC    |
|-----------------|-------|------|---------------|---------------|------------------|------------------|-----------|-------------------|-------------------|-----------|---------|--------|--------|
| A ( $n = 396$ ) | S     | 1    | -1.118        | -0.622        | 100.716          | 40.829           | -34.773   | —                 | —                 | 0.488     | -510.3  | 1042.5 | 1086.3 |
|                 |       | 2    | -1.771        | 2.448         | 2.397            | 2.417            | -0.343    | —                 | —                 | 0.512     |         |        |        |
|                 | SS    | 1    | -1.864        | -2.123        | 41.498           | 1.997            | 38.584    | 0.368             | 0.421             | 0.601     | -492.2* | 1014.3 | 1074   |
|                 |       | 2    | -2.877        | 1.016         | 0.724            | 0.632            | 3.952     | 0.713             | 0.287             | 0.399     |         |        |        |
|                 | C     | 1    | -1.115        | -0.632        | 72.251           | 28.984           | 0         | —                 | —                 | 0.482     | -539.5  | 1101.1 | 1144.9 |
|                 |       | 2    | -1.759        | 2.429         | 2.198            | 2.088            | 0.269     | —                 | —                 | 0.518     |         |        |        |
|                 | SC    | 1    | -1.097        | -0.644        | 101.564          | 38.614           | 0         | -0.995            | -0.001            | 0.48      | -520.3* | 1070.7 | 1130.4 |
|                 |       | 2    | -1.738        | 2.902         | 2.428            | 1.439            | 0.202     | -0.02             | -0.978            | 0.52      |         |        |        |
|                 | WC    | 1    | -1.731        | 2.572         | 0.596            | 0.852            | -0.154    | —                 | —                 | 0.471     | -454.7  | 931.5  | 975.3  |
|                 |       | 2    | -1.1          | -0.681        | 0.932            | 0.895            | -0.333    | —                 | —                 | 0.529     |         |        |        |
|                 | SWC   | 1    | -1.317        | 2.548         | 0.609            | 0.861            | -0.172    | -1                | 0                 | 0.46      | -419.5* | 869    | 928.7  |
|                 |       | 2    | -1.094        | -0.699        | 0.927            | 0.89             | -0.372    | 0                 | 1                 | 0.54      |         |        |        |
| C ( $n = 315$ ) | S     | 1    | -1.938        | 2.22          | 2.488            | 1.457            | -0.304    | —                 | —                 | 0.681     | -650.3  | 1322.6 | 1363.9 |
|                 |       | 2    | -1.128        | -0.656        | 79.955           | 33.057           | -29.051   | —                 | —                 | 0.319     |         |        |        |
|                 | SS    | 1    | -0.424        | 1.198         | 0.103            | 1.415            | -4.736    | -0.08             | 0.92              | 0.557     | -605.7* | 1241.3 | 1297.6 |
|                 |       | 2    | -1.914        | 0.325         | 14.943           | 7.603            | -16.318   | 0                 | -1                | 0.443     |         |        |        |
|                 | C     | 1    | -1.118        | -0.664        | 68.279           | 31.308           | 0         | —                 | —                 | 0.304     | -667.5  | 1356.9 | 1398.2 |
|                 |       | 2    | -1.95         | 2.278         | 2.441            | 1.358            | 0.068     | —                 | —                 | 0.696     |         |        |        |
|                 | SC    | 1    | -1.936        | -3.139        | 2.447            | 0.604            | 0.212     | 0.004             | -0.989            | 0.663     | -659*   | 1347.9 | 1404.2 |
|                 |       | 2    | -1.122        | -0.728        | 41.705           | 14.973           | 0         | 0.02              | 0.953             | 0.337     |         |        |        |
|                 | WC    | 1    | -2.025        | 2.462         | 0.667            | 0.698            | -0.158    | —                 | —                 | 0.597     | -629.4  | 1280.8 | 1322.1 |
|                 |       | 2    | -1.12         | -0.662        | 0.889            | 0.822            | -0.452    | —                 | —                 | 0.403     |         |        |        |
|                 | SWC   | 1    | -2.129        | 2.676         | 0.641            | 0.684            | -0.253    | 0                 | -1                | 0.59      | -604.3* | 1238.5 | 1294.8 |
|                 |       | 2    | -1.104        | -0.685        | 0.887            | 0.825            | -0.448    | -1                | 0                 | 0.41      |         |        |        |
| D ( $n = 398$ ) | S     | 1    | -1.693        | 2.076         | 2.496            | 1.787            | 0.109     | —                 | —                 | 0.576     | -752.8  | 1527.7 | 1571.5 |
|                 |       | 2    | -1.237        | -0.501        | 51.781           | 30.899           | -33.49    | —                 | —                 | 0.424     |         |        |        |
|                 | SS    | 1    | -1.739        | 0.064         | 26.16            | 19.058           | -27.505   | 0                 | -1                | 0.488     | -694.4* | 1418.9 | 1478.7 |
|                 |       | 2    | -0.161        | 0.934         | 0.292            | 0.98             | -4.385    | 0                 | 1                 | 0.512     |         |        |        |
|                 | C     | 1    | -1.69         | 2.015         | 2.709            | 1.092            | 0.351     | —                 | —                 | 0.62      | -800.4  | 1622.8 | 1666.7 |
|                 |       | 2    | -1.166        | -0.601        | 34.994           | 19.676           | 0         | —                 | —                 | 0.38      |         |        |        |
|                 | SC    | 1    | -1.201        | -0.618        | 23.089           | 18.874           | 0         | 0.781             | 0.171             | 0.368     | -791.2* | 1612.5 | 1672.3 |
|                 |       | 2    | -1.575        | -3.137        | 2.573            | 0.048            | 0.544     | 0                 | -0.997            | 0.632     |         |        |        |
|                 | WC    | 1    | -1.17         | -0.619        | 0.834            | 0.781            | -0.618    | —                 | —                 | 0.495     | -746.8  | 1515.5 | 1559.4 |
|                 |       | 2    | -1.511        | 2.183         | 0.7              | 0.67             | 0.279     | —                 | —                 | 0.505     |         |        |        |
|                 | SWC   | 1    | -1.319        | 2.294         | 0.702            | 0.686            | 0.315     | -1                | 0                 | 0.487     | -697.3* | 1424.5 | 1484.3 |
|                 |       | 2    | -1.132        | -0.681        | 0.826            | 0.78             | -0.629    | 0                 | 1                 | 0.513     |         |        |        |

Table S1: Parameter estimation for each component, log-likelihood (LL), AIC and BIC of the mixture of Sine (S), Cosine (C) and wrapped Cauchy (WC) distributions and their sine-skewed versions (respectively, SS, SC, SWC). In the LL value of the sine-skewed models, an asterisk (\*) indicates when the null hypothesis of symmetry is rejected against the sine-skewed version at the level  $\alpha = 0.01$ . Each block corresponds to one amino acid type, from top to bottom: alanine (A), cysteine (C) and aspartic acid (D).

|                 | Model | Comp | $\hat{\mu}_1$ | $\hat{\mu}_2$ | $\hat{\kappa}_1$ | $\hat{\kappa}_2$ | $\hat{r}$ | $\hat{\lambda}_1$ | $\hat{\lambda}_2$ | $\hat{p}$ | LL      | AIC    | BIC    |
|-----------------|-------|------|---------------|---------------|------------------|------------------|-----------|-------------------|-------------------|-----------|---------|--------|--------|
| E ( $n = 396$ ) | S     | 1    | -1.802        | 2.287         | 2.752            | 1.89             | -0.232    | —                 | —                 | 0.513     | -573.8  | 1169.5 | 1213.3 |
|                 |       | 2    | -1.159        | -0.589        | 75.887           | 34.314           | -30.109   | —                 | —                 | 0.487     |         |        |        |
|                 | SS    | 1    | -1.948        | 0.511         | 22.682           | 8.44             | -24.491   | 0                 | -1                | 0.554     | -525.8* | 1081.7 | 1141.4 |
|                 |       | 2    | -0.321        | 1.236         | 0.347            | 2.15             | -5.789    | -0.007            | 0.993             | 0.446     |         |        |        |
|                 | C     | 1    | -1.198        | -0.576        | 25.441           | 15.7             | 0         | —                 | —                 | 0.534     | -619.1  | 1260.2 | 1304   |
|                 |       | 2    | -1.855        | 2.335         | 2.151            | 2.24             | 0.522     | —                 | —                 | 0.466     |         |        |        |
|                 | SC    | 1    | -2.311        | 2.273         | 1.738            | 3.562            | 0.498     | 0.993             | 0.004             | 0.48      | -615.9  | 1261.8 | 1321.5 |
|                 |       | 2    | -1.177        | -0.651        | 20.022           | 17.758           | 0         | -0.002            | 0.992             | 0.52      |         |        |        |
|                 | WC    | 1    | -1.876        | 2.456         | 0.654            | 0.797            | -0.041    | —                 | —                 | 0.457     | -543.5  | 1109   | 1152.8 |
|                 |       | 2    | -1.139        | -0.659        | 0.917            | 0.879            | -0.305    | —                 | —                 | 0.543     |         |        |        |
|                 | SWC   | 1    | -2.248        | 2.488         | 0.65             | 0.804            | -0.141    | 1                 | 0                 | 0.442     | -509*   | 1048.1 | 1107.8 |
|                 |       | 2    | -1.133        | -0.681        | 0.911            | 0.874            | -0.333    | 0                 | 1                 | 0.558     |         |        |        |
| F ( $n = 384$ ) | S     | 1    | -1.455        | -0.264        | 62.806           | 36.62            | -53.242   | —                 | —                 | 0.378     | -668.6  | 1359.1 | 1402.6 |
|                 |       | 2    | -1.935        | 2.391         | 3.163            | 3.835            | -0.385    | —                 | —                 | 0.622     |         |        |        |
|                 | SS    | 1    | -1.69         | 0.071         | 36.673           | 18.314           | -33.72    | 0                 | -1                | 0.394     | -567.7* | 1165.4 | 1224.6 |
|                 |       | 2    | 2.798         | 1.028         | 0.106            | 1.074            | 6.389     | 0                 | 1                 | 0.606     |         |        |        |
|                 | C     | 1    | -1.093        | -0.744        | 101.157          | 46.868           | 0         | —                 | —                 | 0.29      | -707.4  | 1436.7 | 1480.2 |
|                 |       | 2    | -1.908        | 2.212         | 3.495            | 1.764            | 0.068     | —                 | —                 | 0.71      |         |        |        |
|                 | SC    | 1    | -2.203        | 2.226         | 2.696            | 1.791            | 0.233     | 1                 | 0                 | 0.745     | -699*   | 1427.9 | 1487.2 |
|                 |       | 2    | -1.06         | -0.742        | 48.495           | 57.394           | 0         | -0.999            | 0                 | 0.255     |         |        |        |
|                 | WC    | 1    | -1.112        | -0.729        | 0.88             | 0.84             | -0.62     | —                 | —                 | 0.371     | -624.1  | 1270.2 | 1313.7 |
|                 |       | 2    | -2.014        | 2.458         | 0.722            | 0.792            | -0.118    | —                 | —                 | 0.629     |         |        |        |
|                 | SWC   | 1    | -2.229        | 2.491         | 0.707            | 0.801            | -0.14     | 1                 | 0                 | 0.609     | -594*   | 1217.9 | 1277.2 |
|                 |       | 2    | -1.091        | -0.761        | 0.865            | 0.821            | -0.653    | 0                 | 1                 | 0.391     |         |        |        |
| H ( $n = 359$ ) | S     | 1    | -1.234        | -0.554        | 45.984           | 29.88            | -30.744   | —                 | —                 | 0.386     | -723.1  | 1468.2 | 1510.9 |
|                 |       | 2    | -1.944        | 2.144         | 2.351            | 1.903            | -0.13     | —                 | —                 | 0.614     |         |        |        |
|                 | SS    | 1    | -1.718        | -0.003        | 29.748           | 21.5             | -31.047   | 0                 | -1                | 0.449     | -627.2* | 1284.5 | 1342.7 |
|                 |       | 2    | -0.379        | 1.137         | 0.045            | 1.704            | -4.809    | -0.184            | 0.816             | 0.551     |         |        |        |
|                 | C     | 1    | -1.936        | 2.033         | 2.566            | 1.399            | 0.082     | —                 | —                 | 0.656     | -757.7  | 1537.4 | 1580.2 |
|                 |       | 2    | -1.128        | -0.676        | 46.501           | 16.515           | 0         | —                 | —                 | 0.344     |         |        |        |
|                 | SC    | 1    | -1.838        | 2.95          | 2.62             | 0.105            | 0.559     | -0.002            | -0.997            | 0.696     | -719.4* | 1468.9 | 1527.1 |
|                 |       | 2    | -1.09         | -0.674        | 81.691           | 26.537           | 0         | -0.053            | -0.929            | 0.304     |         |        |        |
|                 | WC    | 1    | -2.014        | 2.358         | 0.692            | 0.708            | -0.096    | —                 | —                 | 0.569     | -690.7  | 1403.5 | 1446.2 |
|                 |       | 2    | -1.139        | -0.687        | 0.858            | 0.835            | -0.559    | —                 | —                 | 0.431     |         |        |        |
|                 | SWC   | 1    | -2.068        | 2.542         | 0.688            | 0.701            | -0.114    | 0.076             | -0.924            | 0.566     | -655.7* | 1341.4 | 1399.7 |
|                 |       | 2    | -1.116        | -0.721        | 0.857            | 0.835            | -0.562    | 0                 | 1                 | 0.434     |         |        |        |

Table S2: Parameter estimation for each component, log-likelihood (LL), AIC and BIC of the mixture of Sine (S), Cosine (C) and wrapped Cauchy (WC) distributions and their sine-skewed versions (respectively, SS, SC, SWC). In the LL value of the sine-skewed models, an asterisk (\*) indicates when the null hypothesis of symmetry is rejected against the sine-skewed version at the level  $\alpha = 0.01$ . Each block corresponds to one amino acid type, from top to bottom: glutamic acid (E), phenylalanine (F) and histidine (H).

|                 | Model | Comp | $\hat{\mu}_1$ | $\hat{\mu}_2$ | $\hat{\kappa}_1$ | $\hat{\kappa}_2$ | $\hat{r}$ | $\hat{\lambda}_1$ | $\hat{\lambda}_2$ | $\hat{p}$ | LL      | AIC    | BIC    |
|-----------------|-------|------|---------------|---------------|------------------|------------------|-----------|-------------------|-------------------|-----------|---------|--------|--------|
| I ( $n = 392$ ) | S     | 1    | -1.868        | 2.263         | 7.57             | 13.22            | -1.532    | —                 | —                 | 0.653     | -383.8  | 789.6  | 833.3  |
|                 |       | 2    | -1.202        | -0.656        | 21.263           | 25.604           | -11.431   | —                 | —                 | 0.347     |         |        |        |
|                 | SS    | 1    | -1.229        | -0.631        | 21.297           | 25.636           | -11.855   | 0.295             | -0.332            | 0.347     | -383.1  | 796.2  | 855.8  |
|                 |       | 2    | -1.814        | 2.203         | 7.475            | 12.747           | -1.685    | -0.305            | 0.695             | 0.653     |         |        |        |
|                 | C     | 1    | -1.867        | 2.265         | 6.06             | 10.755           | 0.44      | —                 | —                 | 0.64      | -411.2  | 844.4  | 888.1  |
|                 |       | 2    | -1.203        | -0.642        | 13.575           | 16.828           | 0         | —                 | —                 | 0.36      |         |        |        |
|                 | SC    | 1    | -1.151        | -0.638        | 11.654           | 20.662           | 0         | -0.52             | -0.469            | 0.341     | -407.7  | 845.4  | 904.9  |
|                 |       | 2    | -2.04         | 2.263         | 5.311            | 14.48            | 0.14      | 0.995             | 0.003             | 0.659     |         |        |        |
|                 | WC    | 1    | -1.953        | 2.247         | 0.788            | 0.862            | -0.098    | —                 | —                 | 0.671     | -398.5  | 819    | 862.7  |
|                 |       | 2    | -1.112        | -0.737        | 0.929            | 0.91             | -0.275    | —                 | —                 | 0.329     |         |        |        |
|                 | SWC   | 1    | -1.106        | -0.75         | 0.928            | 0.911            | -0.283    | -0.193            | 0.807             | 0.33      | -372.4* | 774.9  | 834.4  |
|                 |       | 2    | -2.067        | 2.256         | 0.793            | 0.862            | -0.103    | 1                 | 0                 | 0.67      |         |        |        |
| K ( $n = 395$ ) | S     | 1    | -1.104        | -0.671        | 87.458           | 51.645           | -29.964   | —                 | —                 | 0.336     | -732.3  | 1486.5 | 1530.3 |
|                 |       | 2    | -1.797        | 2.208         | 2.887            | 1.369            | -0.313    | —                 | —                 | 0.664     |         |        |        |
|                 | SS    | 1    | -1.371        | -0.448        | 17.963           | 17.442           | -13.505   | 0.554             | -0.446            | 0.459     | -636.2* | 1302.4 | 1362.1 |
|                 |       | 2    | -0.333        | 1.156         | 0.284            | 1.745            | -5.876    | -0.068            | 0.932             | 0.541     |         |        |        |
|                 | C     | 1    | -1.106        | -0.675        | 52.425           | 42.307           | 0         | —                 | —                 | 0.348     | -746.5  | 1514.9 | 1558.7 |
|                 |       | 2    | -1.794        | 2.255         | 2.72             | 1.387            | 0.143     | —                 | —                 | 0.652     |         |        |        |
|                 | SC    | 1    | -1.735        | -3.141        | 2.751            | 0.225            | 0.6       | 0.008             | -0.984            | 0.665     | -726.8* | 1483.7 | 1543.4 |
|                 |       | 2    | -1.086        | -0.684        | 58.789           | 60.593           | 0         | -0.987            | 0.008             | 0.335     |         |        |        |
|                 | WC    | 1    | -1.115        | -0.7          | 0.89             | 0.864            | -0.433    | —                 | —                 | 0.448     | -633.5  | 1289   | 1332.8 |
|                 |       | 2    | -1.855        | 2.432         | 0.712            | 0.81             | -0.024    | —                 | —                 | 0.552     |         |        |        |
|                 | SWC   | 1    | -1.544        | 2.428         | 0.679            | 0.824            | -0.061    | -1                | 0                 | 0.527     | -608.1* | 1246.3 | 1306   |
|                 |       | 2    | -1.103        | -0.725        | 0.873            | 0.848            | -0.497    | 0                 | 1                 | 0.473     |         |        |        |
| L ( $n = 397$ ) | S     | 1    | -1.748        | 2.304         | 4.344            | 6.363            | 0.446     | —                 | —                 | 0.592     | -592.6  | 1207.1 | 1251   |
|                 |       | 2    | -1.271        | -0.55         | 21.619           | 19.875           | -15.204   | —                 | —                 | 0.408     |         |        |        |
|                 | SS    | 1    | -2.023        | 0.158         | 15.134           | 16.828           | -23.745   | 1                 | 0                 | 0.411     | -558.2* | 1146.4 | 1206.2 |
|                 |       | 2    | -0.199        | 0.91          | 0.17             | 1.11             | -7.13     | 0                 | 1                 | 0.589     |         |        |        |
|                 | C     | 1    | -1.74         | 2.313         | 4.914            | 7.795            | 0.51      | —                 | —                 | 0.553     | -642.3  | 1306.7 | 1350.5 |
|                 |       | 2    | -1.234        | -0.551        | 5.802            | 8.742            | 0         | —                 | —                 | 0.447     |         |        |        |
|                 | SC    | 1    | -1.726        | 2.5           | 3.329            | 4.267            | 1.38      | 0                 | -0.996            | 0.582     | -629.4* | 1288.8 | 1348.5 |
|                 |       | 2    | -1.237        | -0.678        | 8.952            | 9.668            | 0         | 0.01              | 0.989             | 0.418     |         |        |        |
|                 | WC    | 1    | -1.129        | -0.704        | 0.894            | 0.868            | -0.514    | —                 | —                 | 0.389     | -572.8  | 1167.6 | 1211.4 |
|                 |       | 2    | -1.78         | 2.349         | 0.742            | 0.819            | 0.013     | —                 | —                 | 0.611     |         |        |        |
|                 | SWC   | 1    | -1.779        | 2.439         | 0.743            | 0.802            | 0         | 0                 | -1                | 0.618     | -549.6* | 1129.2 | 1189   |
|                 |       | 2    | -1.113        | -0.731        | 0.898            | 0.875            | -0.502    | 0                 | 1                 | 0.382     |         |        |        |

Table S3: Parameter estimation for each component, log-likelihood (LL), AIC and BIC of the mixture of Sine (S), Cosine (C) and wrapped Cauchy (WC) distributions and their sine-skewed versions (respectively, SS, SC, SWC). In the LL value of the sine-skewed models, an asterisk (\*) indicates when the null hypothesis of symmetry is rejected against the sine-skewed version at the level  $\alpha = 0.01$ . Each block corresponds to one amino acid type, from top to bottom: isoleucine (I), lysine (K) and leucine (L).

|                 | Model | Comp | $\hat{\mu}_1$ | $\hat{\mu}_2$ | $\hat{\kappa}_1$ | $\hat{\kappa}_2$ | $\hat{\tau}$ | $\hat{\lambda}_1$ | $\hat{\lambda}_2$ | $\hat{p}$ | LL      | AIC    | BIC    |
|-----------------|-------|------|---------------|---------------|------------------|------------------|--------------|-------------------|-------------------|-----------|---------|--------|--------|
| M ( $n = 358$ ) | S     | 1    | -1.114        | -0.677        | 143.18           | 60.967           | -38.71       | —                 | —                 | 0.404     | -497.3  | 1016.6 | 1059.3 |
|                 |       | 2    | -1.861        | 2.181         | 3.369            | 1.618            | -0.793       | —                 | —                 | 0.596     |         |        |        |
|                 | SS    | 1    | -1.865        | 2.723         | 3.171            | 1.097            | -0.49        | 0                 | -1                | 0.544     | -478.5* | 987    | 1045.2 |
|                 |       | 2    | -1.733        | 0.896         | 110.398          | 0.087            | -79.524      | -0.105            | -0.837            | 0.456     |         |        |        |
|                 | C     | 1    | -1.104        | -0.633        | 19.305           | 27.605           | 6.058        | —                 | —                 | 0.465     | -573.3  | 1168.5 | 1211.2 |
|                 |       | 2    | -1.925        | 2.272         | 3.133            | 2.359            | 0            | —                 | —                 | 0.535     |         |        |        |
|                 | SC    | 1    | -1.144        | -0.681        | 37.525           | 75.936           | 0            | 0.924             | 0.018             | 0.415     | -535.3* | 1100.6 | 1158.8 |
|                 |       | 2    | -1.863        | -3.14         | 2.729            | 0.642            | 0.213        | -0.009            | -0.989            | 0.585     |         |        |        |
|                 | WC    | 1    | -1.964        | 2.435         | 0.701            | 0.785            | -0.208       | —                 | —                 | 0.52      | -450    | 922.1  | 964.8  |
|                 |       | 2    | -1.115        | -0.688        | 0.923            | 0.907            | -0.397       | —                 | —                 | 0.48      |         |        |        |
|                 | SWC   | 1    | -2.252        | 2.515         | 0.657            | 0.779            | -0.313       | 1                 | 0                 | 0.505     | -429.4* | 888.8  | 947    |
|                 |       | 2    | -1.108        | -0.7          | 0.915            | 0.899            | -0.433       | 0                 | 1                 | 0.495     |         |        |        |
| N ( $n = 397$ ) | S     | 1    | -1.788        | 1.288         | 4.168            | 0.911            | -0.679       | —                 | —                 | 0.677     | -877.6  | 1777.1 | 1820.9 |
|                 |       | 2    | -0.039        | -0.035        | 11.995           | 49.093           | 40.82        | —                 | —                 | 0.323     |         |        |        |
|                 | SS    | 1    | -1.637        | -0.039        | 19.373           | 14.888           | -17.886      | 0.289             | -0.711            | 0.478     | -844.5* | 1719   | 1778.8 |
|                 |       | 2    | -0.361        | 1.051         | 0.249            | 1.821            | -3.64        | -0.057            | 0.943             | 0.522     |         |        |        |
|                 | C     | 1    | -0.868        | -0.231        | 0                | 3.543            | 1.927        | —                 | —                 | 0.53      | -1050.9 | 2123.8 | 2167.6 |
|                 |       | 2    | -1.88         | 1.933         | 5.111            | 1.88             | 0.006        | —                 | —                 | 0.47      |         |        |        |
|                 | SC    | 1    | -1.126        | -0.635        | 124.929          | 60.021           | 0            | 0.004             | -0.24             | 0.211     | -962.2* | 1954.5 | 2014.2 |
|                 |       | 2    | -1.73         | 2.698         | 1.534            | 0                | 0.22         | 0.047             | -0.953            | 0.789     |         |        |        |
|                 | WC    | 1    | -1.247        | -0.474        | 0.771            | 0.691            | -0.672       | —                 | —                 | 0.519     | -931.4  | 1884.9 | 1928.7 |
|                 |       | 2    | -1.761        | 1.974         | 0.678            | 0.548            | 0.193        | —                 | —                 | 0.481     |         |        |        |
|                 | SWC   | 1    | -1.17         | -0.593        | 0.751            | 0.673            | -0.674       | 0.039             | 0.961             | 0.571     | -883.8* | 1797.7 | 1857.4 |
|                 |       | 2    | -1.732        | 2.446         | 0.72             | 0.58             | -0.122       | -0.208            | -0.792            | 0.429     |         |        |        |
| Q ( $n = 390$ ) | S     | 1    | -1.142        | -0.629        | 112.069          | 46.009           | -48.609      | —                 | —                 | 0.475     | -556.7  | 1135.4 | 1179   |
|                 |       | 2    | -1.783        | 2.2           | 2.722            | 1.493            | -0.261       | —                 | —                 | 0.525     |         |        |        |
|                 | SS    | 1    | -0.295        | 1.271         | 0.27             | 2.214            | -5.189       | -0.114            | 0.886             | 0.431     | -554.1  | 1138.2 | 1197.7 |
|                 |       | 2    | -1.925        | 0.345         | 21.339           | 11.085           | -24.173      | 0                 | -1                | 0.569     |         |        |        |
|                 | C     | 1    | -1.711        | -3.142        | 2.786            | 0.131            | 0.299        | —                 | —                 | 0.594     | -636.7  | 1295.3 | 1338.9 |
|                 |       | 2    | -1.106        | -0.696        | 125.88           | 101.793          | 0            | —                 | —                 | 0.406     |         |        |        |
|                 | SC    | 1    | -1.785        | -3.142        | 2.882            | 0.627            | 0.007        | 0                 | -0.999            | 0.531     | -578.5* | 1187.1 | 1246.6 |
|                 |       | 2    | -1.118        | -0.647        | 84.012           | 32.417           | 0            | -0.638            | -0.362            | 0.469     |         |        |        |
|                 | WC    | 1    | -1.762        | 2.404         | 0.665            | 0.784            | 0            | —                 | —                 | 0.442     | -512.6  | 1047.2 | 1090.8 |
|                 |       | 2    | -1.127        | -0.691        | 0.906            | 0.877            | -0.494       | —                 | —                 | 0.558     |         |        |        |
|                 | SWC   | 1    | -1.116        | -0.712        | 0.892            | 0.861            | -0.543       | 0                 | 1                 | 0.583     | -479.1* | 988.2  | 1047.7 |
|                 |       | 2    | -1.405        | 2.415         | 0.648            | 0.803            | -0.12        | -1                | 0                 | 0.417     |         |        |        |

Table S4: Parameter estimation for each component, log-likelihood (LL), AIC and BIC of the mixture of Sine (S), Cosine (C) and wrapped Cauchy (WC) distributions and their sine-skewed versions (respectively, SS, SC, SWC). In the LL value of the sine-skewed models, an asterisk (\*) indicates when the null hypothesis of symmetry is rejected against the sine-skewed version at the level  $\alpha = 0.01$ . Each block corresponds to one amino acid type, from top to bottom: methionine (M), asparagine (N) and glutamine (Q).

|                 | Model | Comp | $\hat{\mu}_1$ | $\hat{\mu}_2$ | $\hat{\kappa}_1$ | $\hat{\kappa}_2$ | $\hat{r}$ | $\hat{\lambda}_1$ | $\hat{\lambda}_2$ | $\hat{p}$ | LL      | AIC    | BIC    |
|-----------------|-------|------|---------------|---------------|------------------|------------------|-----------|-------------------|-------------------|-----------|---------|--------|--------|
| R ( $n = 386$ ) | S     | 1    | -1.865        | 2.091         | 2.963            | 1.257            | -0.279    | —                 | —                 | 0.636     | -662.4  | 1346.8 | 1390.3 |
|                 |       | 2    | -1.099        | -0.68         | 123.755          | 56.812           | -45.301   | —                 | —                 | 0.364     |         |        |        |
|                 | SS    | 1    | -0.347        | 1.106         | 0.048            | 1.334            | -5.417    | -0.201            | 0.799             | 0.501     | -566.1* | 1162.2 | 1221.5 |
|                 |       | 2    | -1.727        | 0.056         | 35.661           | 23.875           | -37.145   | 0                 | -1                | 0.499     |         |        |        |
|                 | C     | 1    | -1.112        | -0.692        | 79.373           | 39.013           | 0         | —                 | —                 | 0.379     | -681.4  | 1384.8 | 1428.3 |
|                 |       | 2    | -1.879        | 2.199         | 2.903            | 0.942            | 0.332     | —                 | —                 | 0.621     |         |        |        |
|                 | SC    | 1    | -1.85         | -3.142        | 2.945            | 0                | 0.604     | 0.016             | -0.984            | 0.633     | -657.5* | 1344.9 | 1404.3 |
|                 |       | 2    | -1.1          | -0.709        | 75.48            | 34.949           | 0         | 0                 | 1                 | 0.367     |         |        |        |
|                 | WC    | 1    | -1.105        | -0.701        | 0.885            | 0.865            | -0.568    | —                 | —                 | 0.483     | -595.8  | 1213.7 | 1257.2 |
|                 |       | 2    | -1.998        | 2.426         | 0.724            | 0.768            | -0.075    | —                 | —                 | 0.517     |         |        |        |
|                 | SWC   | 1    | -1.089        | -0.725        | 0.884            | 0.867            | -0.576    | 0                 | 1                 | 0.482     | -564.2* | 1158.3 | 1217.6 |
|                 |       | 2    | -1.995        | 2.557         | 0.723            | 0.757            | -0.032    | 0                 | -1                | 0.518     |         |        |        |
| T ( $n = 392$ ) | S     | 1    | -1.915        | 2.597         | 5.577            | 8.326            | -0.686    | —                 | —                 | 0.633     | -622.9  | 1267.8 | 1311.5 |
|                 |       | 2    | -1.478        | -0.418        | 8.282            | 12.405           | -7.424    | —                 | —                 | 0.367     |         |        |        |
|                 | SS    | 1    | -1.62         | -0.244        | 13.809           | 16.211           | -14.233   | 0                 | -1                | 0.362     | -616.5* | 1263   | 1322.6 |
|                 |       | 2    | -2.144        | 2.616         | 4.317            | 6.822            | -0.613    | 1                 | 0                 | 0.638     |         |        |        |
|                 | C     | 1    | -1.887        | 2.561         | 5.839            | 7.902            | 0.234     | —                 | —                 | 0.616     | -661.1  | 1344.2 | 1387.9 |
|                 |       | 2    | -1.461        | -0.447        | 4.813            | 7.018            | 0         | —                 | —                 | 0.384     |         |        |        |
|                 | SC    | 1    | -1.578        | -0.441        | 4.853            | 7.639            | 0         | 0.68              | 0.263             | 0.377     | -656.7  | 1343.5 | 1403   |
|                 |       | 2    | -2.015        | 2.551         | 4.747            | 7.776            | 0.165     | 0.495             | 0.488             | 0.623     |         |        |        |
|                 | WC    | 1    | -1.194        | -0.643        | 0.838            | 0.812            | -0.639    | —                 | —                 | 0.316     | -682.1  | 1386.2 | 1429.9 |
|                 |       | 2    | -1.984        | 2.595         | 0.748            | 0.763            | 0         | —                 | —                 | 0.684     |         |        |        |
|                 | SWC   | 1    | -2.2          | 2.587         | 0.735            | 0.773            | -0.113    | 1                 | 0                 | 0.661     | -647.1* | 1324.2 | 1383.8 |
|                 |       | 2    | -1.165        | -0.675        | 0.822            | 0.799            | -0.653    | -0.891            | 0.109             | 0.339     |         |        |        |
| V ( $n = 393$ ) | S     | 1    | -1.96         | 2.315         | 7.415            | 14.331           | -2.792    | —                 | —                 | 0.682     | -425.6  | 873.3  | 917    |
|                 |       | 2    | -1.25         | -0.609        | 16.707           | 18.913           | -10.831   | —                 | —                 | 0.318     |         |        |        |
|                 | SS    | 1    | -1.31         | -0.55         | 17.059           | 19.235           | -12.111   | 0.346             | -0.439            | 0.318     | -423.9  | 877.7  | 937.3  |
|                 |       | 2    | -1.963        | 2.378         | 7.41             | 13.627           | -2.712    | -0.144            | -0.855            | 0.682     |         |        |        |
|                 | C     | 1    | -1.968        | 2.327         | 6.624            | 11.321           | 0         | —                 | —                 | 0.676     | -465.3  | 952.5  | 996.2  |
|                 |       | 2    | -1.233        | -0.603        | 9.393            | 10.15            | 0.072     | —                 | —                 | 0.324     |         |        |        |
|                 | SC    | 1    | -1.968        | 2.327         | 6.624            | 11.321           | 0         | -0.015            | -0.03             | 0.676     | -464.6  | 959.3  | 1018.9 |
|                 |       | 2    | -1.233        | -0.603        | 9.393            | 10.15            | 0.072     | -0.394            | -0.446            | 0.324     |         |        |        |
|                 | WC    | 1    | -1.119        | -0.741        | 0.925            | 0.911            | -0.319    | —                 | —                 | 0.295     | -396.9  | 815.8  | 859.5  |
|                 |       | 2    | -2.068        | 2.283         | 0.812            | 0.857            | -0.176    | —                 | —                 | 0.705     |         |        |        |
|                 | SWC   | 1    | -2.148        | 2.298         | 0.81             | 0.857            | -0.189    | 1                 | 0                 | 0.707     | -368.7* | 767.4  | 827    |
|                 |       | 2    | -1.113        | -0.755        | 0.924            | 0.913            | -0.325    | 0                 | 1                 | 0.293     |         |        |        |

Table S5: Parameter estimation for each component, log-likelihood (LL), AIC and BIC of the mixture of Sine (S), Cosine (C) and wrapped Cauchy (WC) distributions and their sine-skewed versions (respectively, SS, SC, SWC). In the LL value of the sine-skewed models, an asterisk (\*) indicates when the null hypothesis of symmetry is rejected against the sine-skewed version at the level  $\alpha = 0.01$ . Each block corresponds to one amino acid type, from top to bottom: arginine (R), threonine (T) and valine (V).



|                 | Model | Comp | $\hat{\mu}_1$ | $\hat{\mu}_2$ | $\hat{\kappa}_1$ | $\hat{\kappa}_2$ | $\hat{r}$ | $\hat{\lambda}_1$ | $\hat{\lambda}_2$ | $\hat{p}$ | LL      | AIC    | BIC    |
|-----------------|-------|------|---------------|---------------|------------------|------------------|-----------|-------------------|-------------------|-----------|---------|--------|--------|
| W ( $n = 325$ ) | S     | 1    | -1.96         | 2.25          | 3.974            | 1.73             | -0.356    | —                 | —                 | 0.578     | -509.6  | 1041.3 | 1082.9 |
|                 |       | 2    | -1.157        | -0.619        | 82.434           | 35.036           | -38.683   | —                 | —                 | 0.422     |         |        |        |
|                 | SS    | 1    | 2.95          | 0.843         | 0.859            | 0.025            | 5.165     | 0.325             | 0.674             | 0.482     | -507.6  | 1045.3 | 1102   |
|                 |       | 2    | -1.826        | 0.25          | 23.739           | 11.417           | -23.517   | 0.003             | -0.996            | 0.518     |         |        |        |
|                 | C     | 1    | -1.951        | 2.229         | 3.812            | 2.174            | 0.173     | —                 | —                 | 0.488     | -590.6  | 1203.2 | 1244.8 |
|                 |       | 2    | -1.212        | -0.62         | 9.336            | 12.046           | 0         | —                 | —                 | 0.512     |         |        |        |
|                 | SC    | 1    | -1.121        | -0.733        | 58.255           | 87.092           | 0         | 0.025             | 0.974             | 0.312     | -545.9* | 1121.7 | 1178.5 |
|                 |       | 2    | -1.833        | -3.142        | 4.057            | 0                | 0.547     | 0.001             | -0.999            | 0.688     |         |        |        |
|                 | WC    | 1    | -2.083        | 2.483         | 0.685            | 0.777            | -0.149    | —                 | —                 | 0.499     | -519.5  | 1060.9 | 1102.6 |
|                 |       | 2    | -1.117        | -0.675        | 0.887            | 0.831            | -0.486    | —                 | —                 | 0.501     |         |        |        |
|                 | SWC   | 1    | -1.098        | -0.701        | 0.877            | 0.824            | -0.519    | -0.597            | 0.403             | 0.516     | -486.5* | 1003.1 | 1059.8 |
|                 |       | 2    | -2.342        | 2.56          | 0.676            | 0.772            | -0.26     | 1                 | 0                 | 0.484     |         |        |        |
| Y ( $n = 392$ ) | S     | 1    | -1.981        | 2.44          | 3.791            | 4.955            | -1.023    | —                 | —                 | 0.611     | -626.7  | 1275.3 | 1319   |
|                 |       | 2    | -1.496        | -0.261        | 52.078           | 35.341           | -47.644   | —                 | —                 | 0.389     |         |        |        |
|                 | SS    | 1    | -0.413        | 1.016         | 0.035            | 0.763            | -5.776    | -0.078            | 0.921             | 0.604     | -581.9* | 1193.9 | 1253.5 |
|                 |       | 2    | -1.586        | -0.125        | 53.682           | 32.413           | -48.834   | -0.001            | -0.996            | 0.396     |         |        |        |
|                 | C     | 1    | -1.098        | -0.72         | 26.022           | 36.381           | 10.621    | —                 | —                 | 0.306     | -729.6  | 1481.2 | 1524.9 |
|                 |       | 2    | -1.987        | 2.264         | 3.736            | 1.398            | 0         | —                 | —                 | 0.694     |         |        |        |
|                 | SC    | 1    | -1.136        | -0.704        | 22.43            | 29.101           | 1.065     | 0.479             | 0.439             | 0.306     | -710.9* | 1451.8 | 1511.3 |
|                 |       | 2    | -1.975        | -3.138        | 3.63             | 1.046            | 0         | -0.005            | -0.992            | 0.694     |         |        |        |
|                 | WC    | 1    | -2.03         | 2.454         | 0.726            | 0.772            | -0.117    | —                 | —                 | 0.653     | -658.1  | 1338.2 | 1381.9 |
|                 |       | 2    | -1.106        | -0.741        | 0.875            | 0.871            | -0.499    | —                 | —                 | 0.347     |         |        |        |
|                 | SWC   | 1    | -2.274        | 2.515         | 0.696            | 0.773            | -0.21     | 1                 | 0                 | 0.629     | -631.1* | 1292.2 | 1351.8 |
|                 |       | 2    | -1.093        | -0.761        | 0.851            | 0.846            | -0.569    | 0                 | 1                 | 0.371     |         |        |        |

Table S6: Parameter estimation for each component, log-likelihood (LL), AIC and BIC of the mixture of Sine (S), Cosine (C) and wrapped Cauchy (WC) distributions and their sine-skewed versions (respectively, SS, SC, SWC). In the LL value of the sine-skewed models, an asterisk (\*) indicates when the null hypothesis of symmetry is rejected against the sine-skewed version at the level  $\alpha = 0.01$ . Each block corresponds to one amino acid type, from top to bottom: tryptophan (W) and tyrosine (Y).

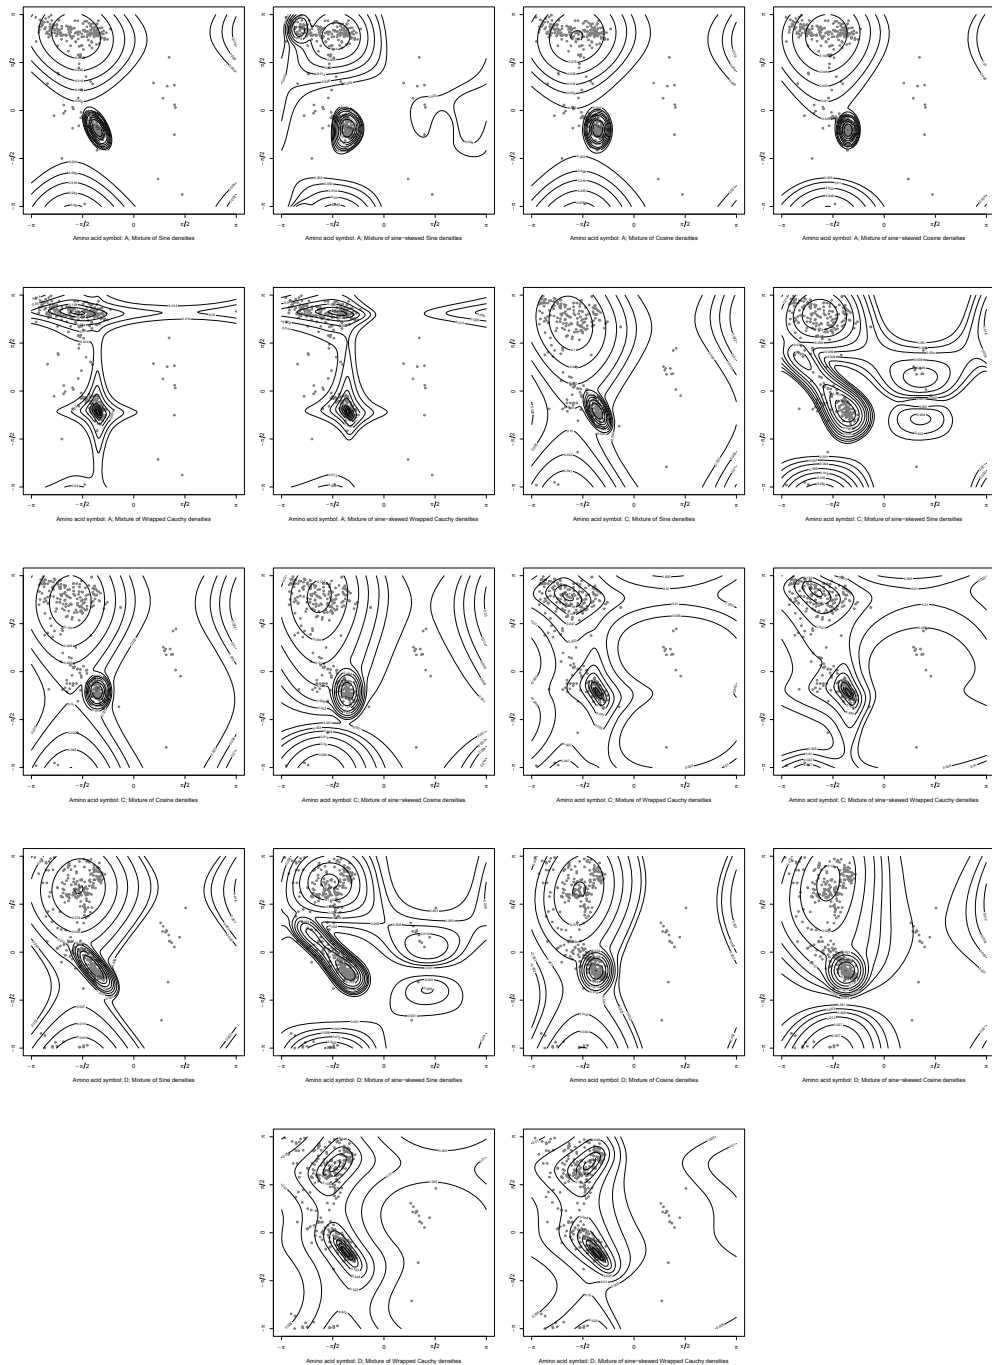

Figure S1: Ramachandran plot (gray points) and maximum likelihood fits (black contour) of mixtures of the base models and of mixtures of their sine-skewed versions for the protein data. The studied amino acid types are: alanine (A), cysteine (C) and aspartic acid (D).

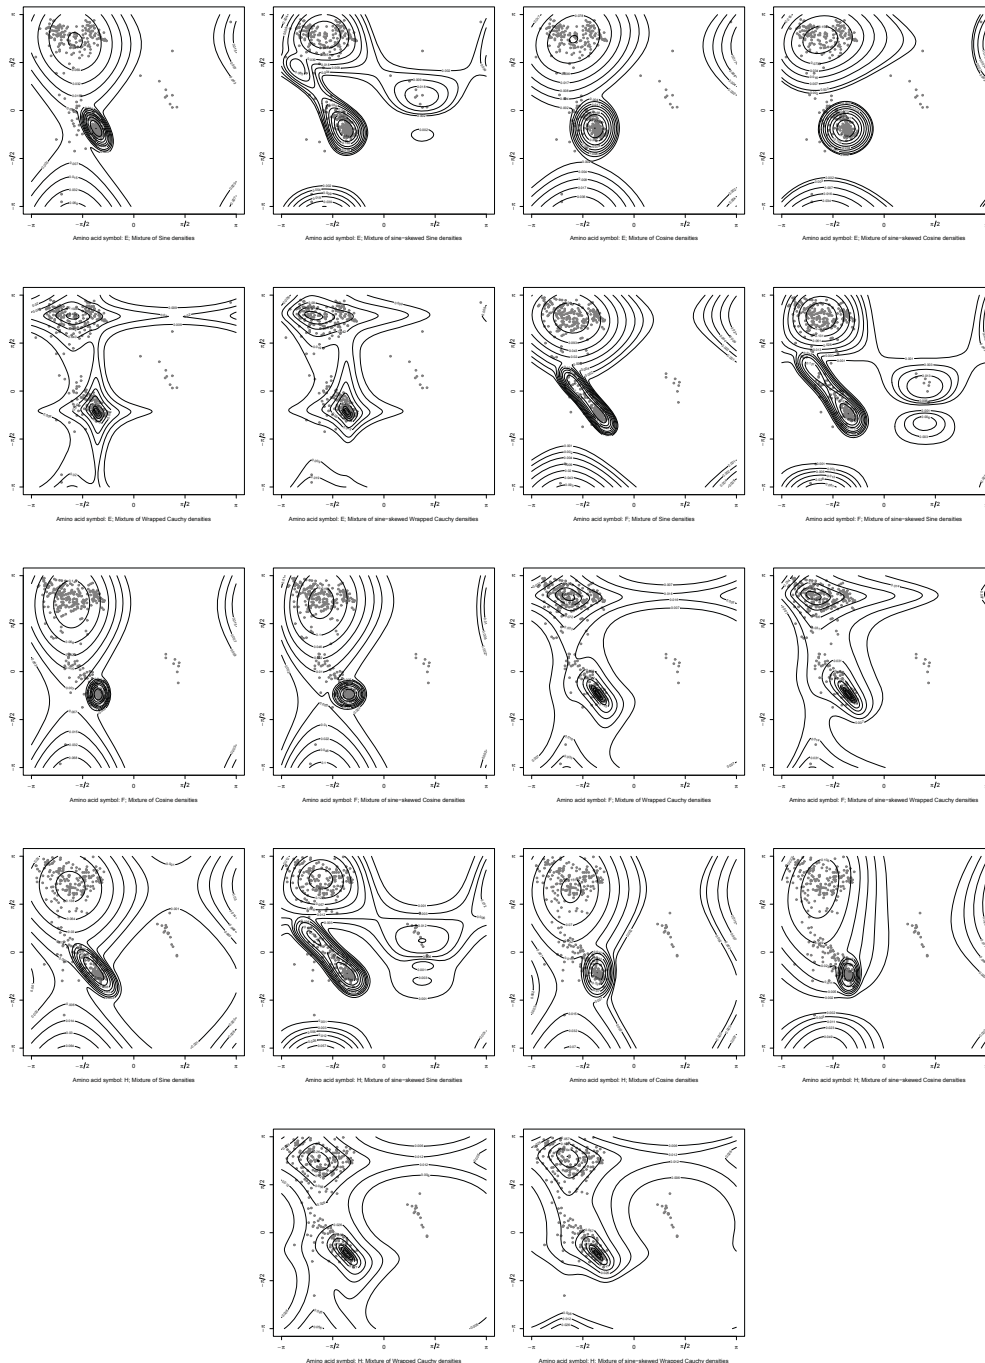

Figure S2: Ramachandran plot (gray points) and maximum likelihood fits (black contour) of mixtures of the base models and of mixtures of their sine-skewed versions for the protein data. The studied amino acid types are: glutamic acid (E), phenylalanine (F) and histidine (H).

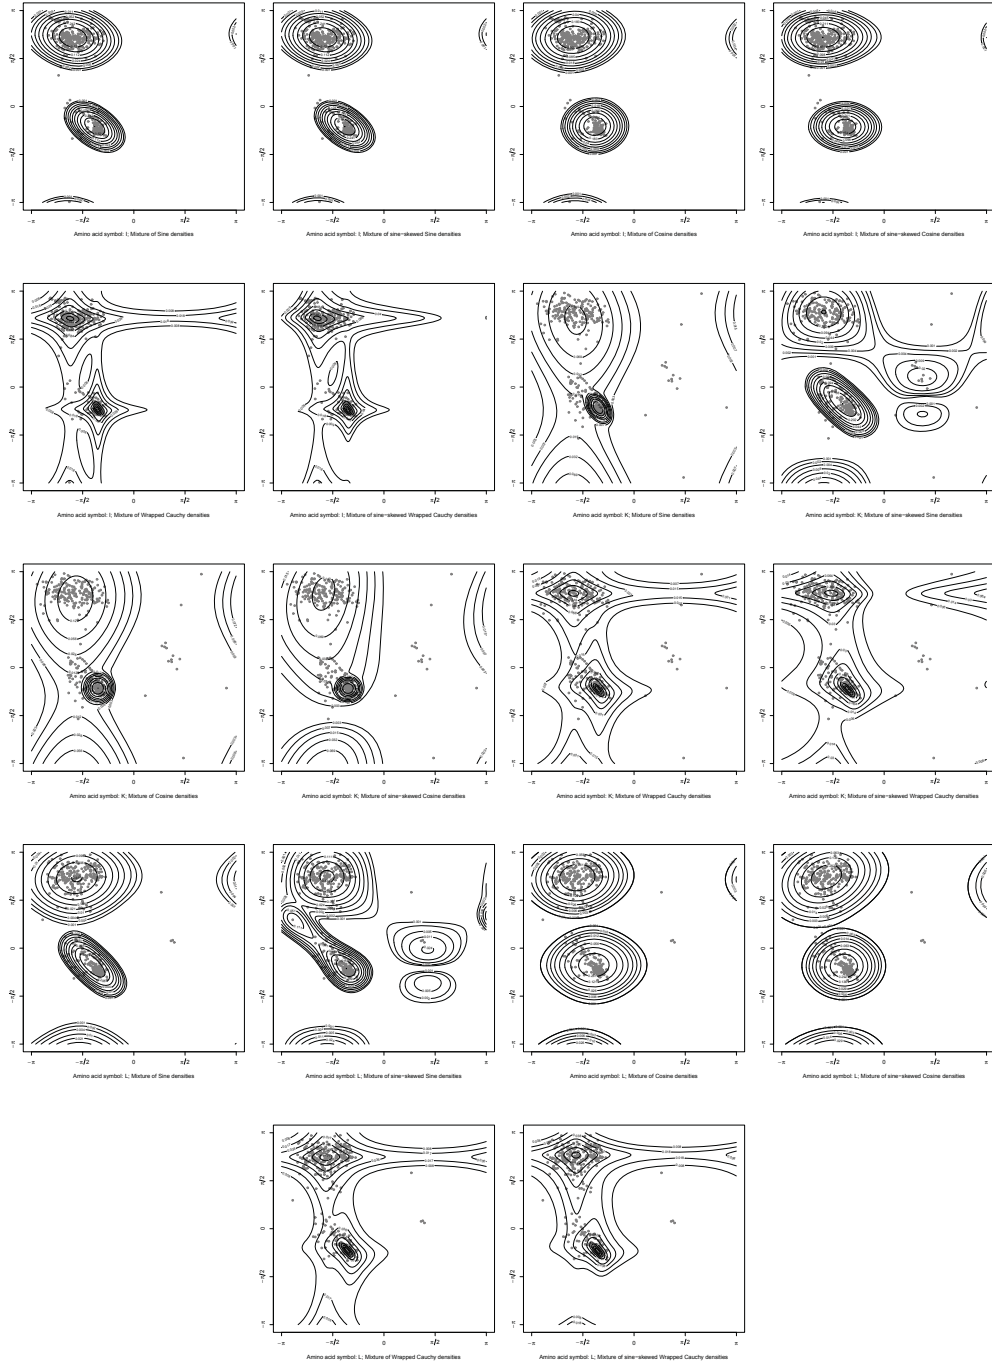

Figure S3: Ramachandran plot (gray points) and maximum likelihood fits (black contour) of mixtures of the base models and of mixtures of their sine-skewed versions for the protein data. The studied amino acid types are: isoleucine (I), lysine (K) and leucine (L).

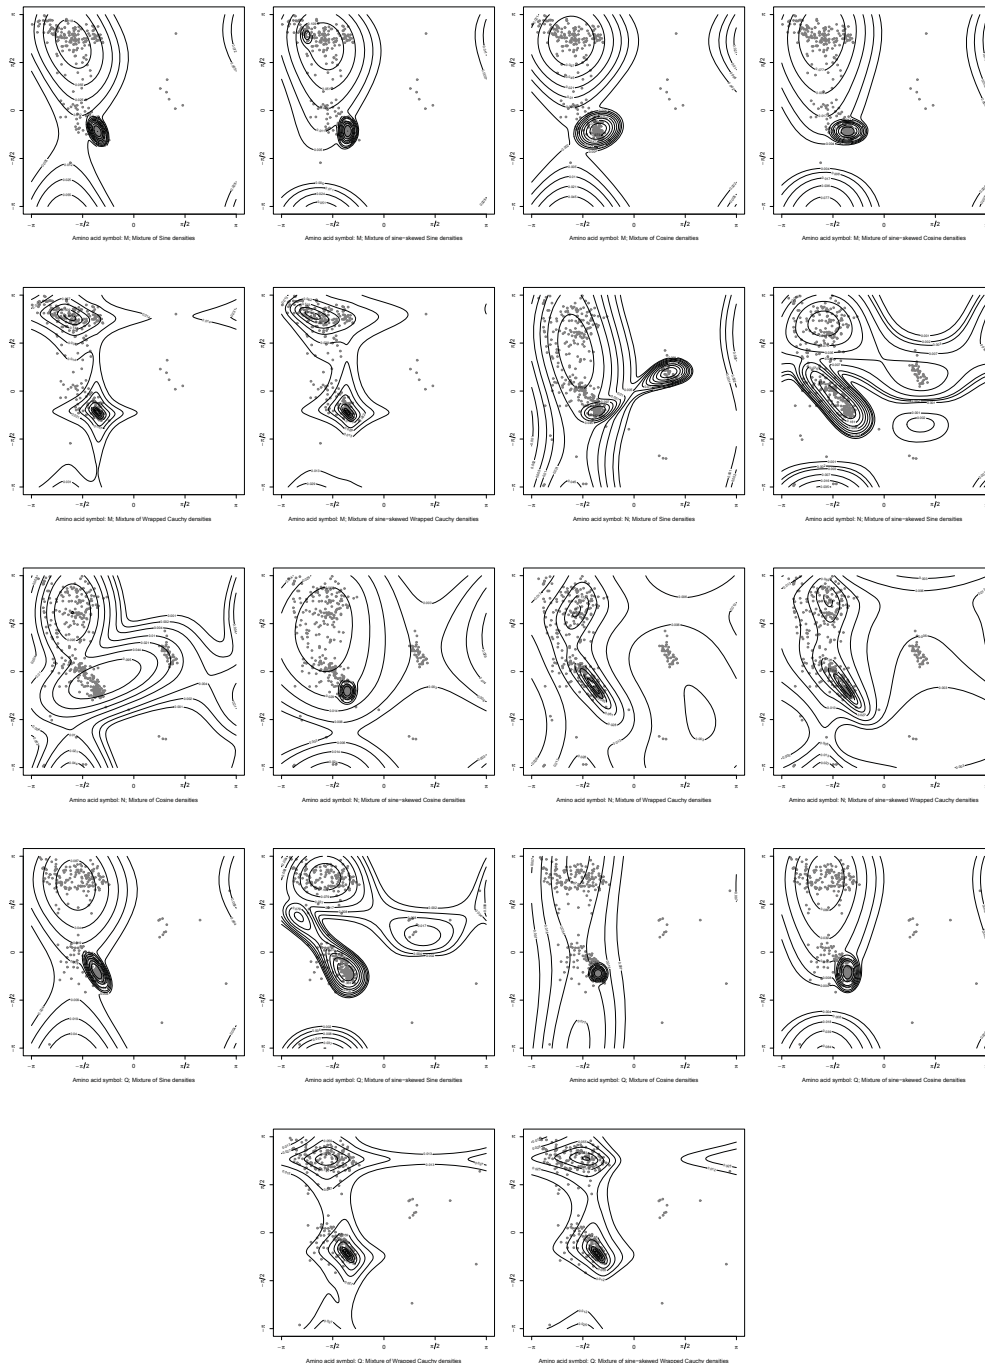

Figure S4: Ramachandran plot (gray points) and maximum likelihood fits (black contour) of mixtures of the base models and of mixtures of their sine-skewed versions for the protein data. The studied amino acid types are: methionine (M), asparagine (N) and glutamine (Q).

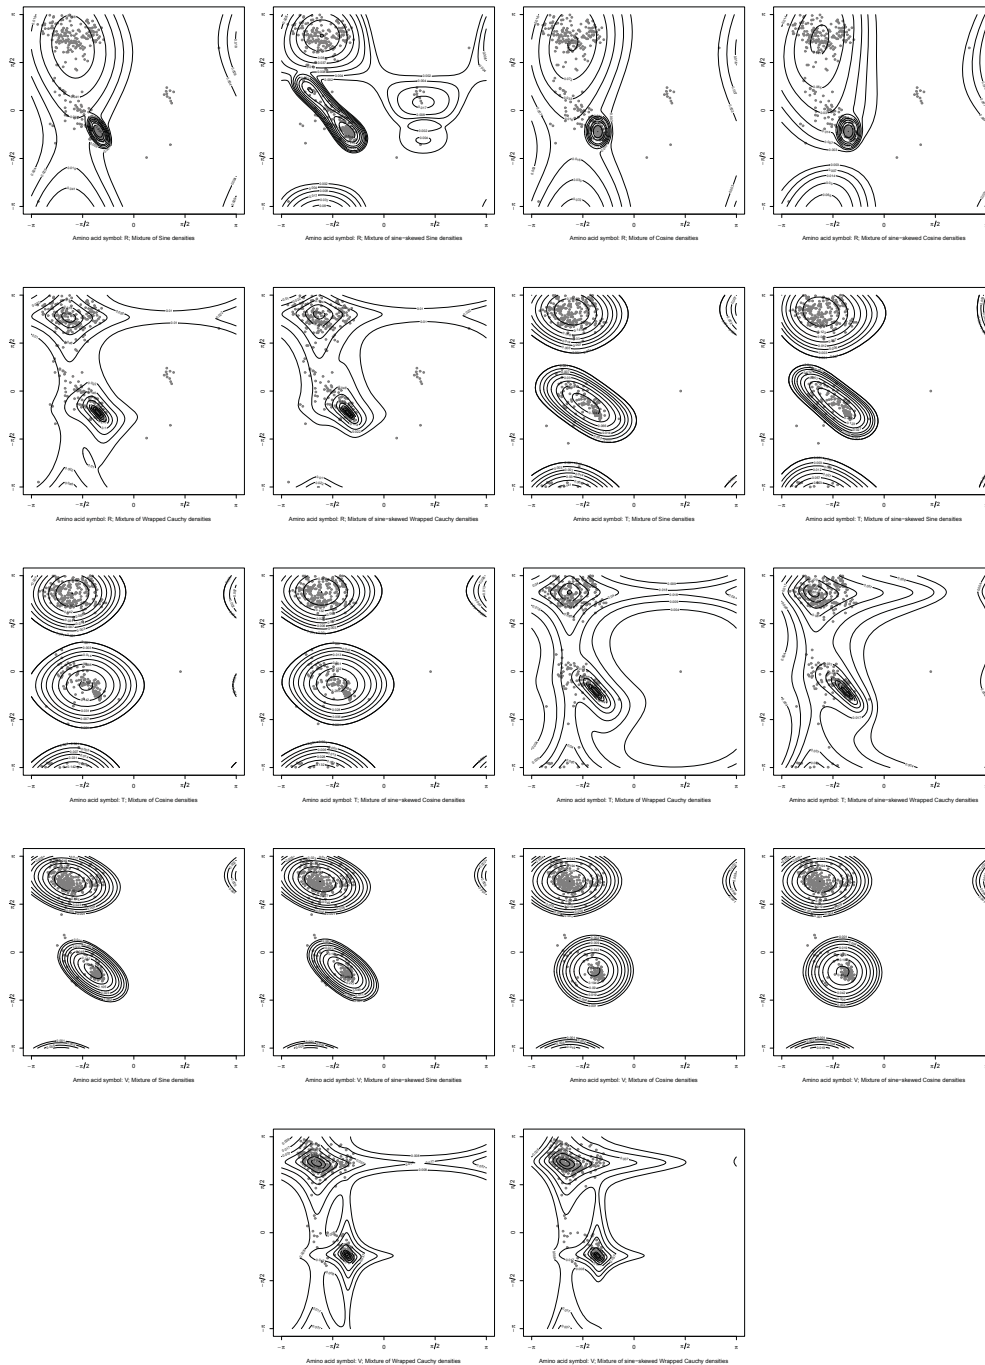

Figure S5: Ramachandran plot (gray points) and maximum likelihood fits (black contour) of mixtures of the base models and of mixtures of their sine-skewed versions for the protein data. The studied amino acid types are: arginine (R), threonine (T) and valine (V).

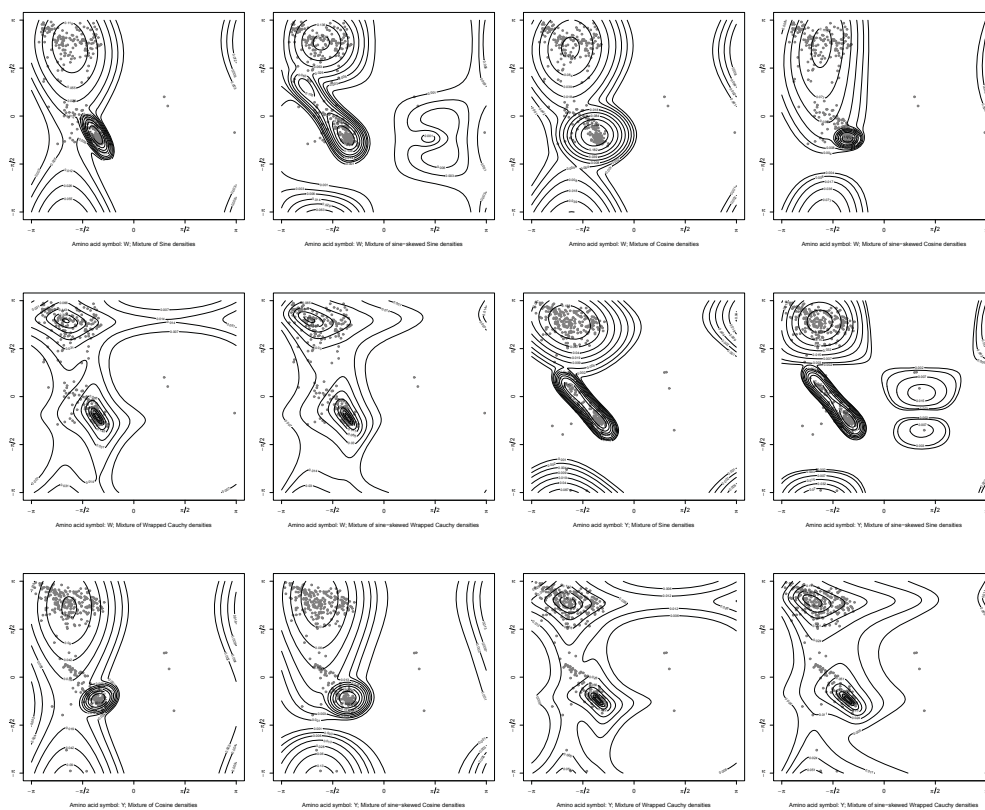

Figure S6: Ramachandran plot (gray points) and maximum likelihood fits (black contour) of mixtures of the base models and of mixtures of their sine-skewed versions for the protein data. The studied amino acid types are: tryptophan (W) and tyrosine (Y).
